# Supplementary material for: QuantAgent: Seeking Holy Grail in Trading by Self-Improving Large Language Model
Source: arXiv:2402.03755 source file (2024-02-06)
Supplement: Supplementary file 1 [file proof.tex]

\section{Proof}

\subsection{Proof of Lemma \ref{lem:rafa_result}}\label{sec:proof_rafa_result}
Proof of lemma \ref{lem:rafa_result} essentially follows that of Theorem 4.4 in \cite{liu_reason_2023}. Here we briefly recite it:

First, we relate the model parameter estimation error with the information gain.

\paragraph{Information gain}
Consider the entropy of the posterior distribution $p_t(\theta)$ at time t:
\begin{equation}
    H_t = - \int p_t(\theta) \log p_t(\theta) d\theta
\end{equation}
$H_t$ is expected to decrease as $t$ increases, meaning that the uncertainty in environment estimation reduces as more observations is attained. Meanwhile, the uncertainty in posterior distribution will be reflected on the estimation error of value function. To reflect this process, we introduce the idea of information coefficient $\Gamma_{t^\dagger}(\delta)$ \citep{abbasi-yadkori_bayesian_2015}, which is the minimum value that makes the following inequality holds for all $t \in \{t^\dagger+1, ..., T-1\}$ with probability at least $1 - \delta$, if $H_{t^\dagger} - H_t \leq \log2$:
\begin{equation}\label{equ:info_coeff}
    | (r_{\theta^*} - r_{\theta_t})(s_t, a_t) + ((P_{\theta^*} - P_{\theta_t})V)(s_t, a_t) | \le \Gamma_{t^\dagger}(\delta) \sqrt{I(\theta;\xi_{t+1}|D_t)},
\end{equation}
where $I(\theta;\xi_{t+1}|D_t) = H_{t+1} - H_t$ is the information gain over  after observing the $t+1$-th step $(s_t, a_t, r_t, s_{t+1})$
Equation \ref{equ:info_coeff} essentially depicts that as the new information gets smaller with more explorations, meaning that the exploration has already gained a lot of information and getting new information is hard, the bound of the estimation error for value function gets smaller. As long as $\Gamma_{t^\dagger}(\delta)$ is finite, the estimation error can be bounded.

According to Eq. C.1 in \cite{liu_reason_2023}, the Bayesian regret in Eq. \ref{equ:bayesian_regret} can be decomposed as:
\begin{align} \label{equ:regret_decomp_1}
    \mathcal{R}(T) & = \mathbb{E}_{\theta \sim p(\theta)}[\sum_{t=1}^{T} V^{\pi^*}_\theta (s_t) - V^{\pi^t}_\theta (s_t)] \notag \\
    & = \mathbb{E}_{\theta \sim p(\theta)}[\sum_{k=1}^{K} \sum_{t=t_k}^{t_{k+1}-1} V^{\text{PL}^*(\theta)}_{\theta} (s_t) - V^{\pi^t}_\theta (s_t)] \notag \\
    & = \underbrace{\mathbb{E}_{\theta \sim p(\theta)}[\sum_{k=1}^{K} \sum_{t=t_k}^{t_{k+1}-1} V^{\text{PL}^*(\theta^k)}_{\theta^k} (s_t) - V^{\pi^k}_{\theta^k} (s_t)]}_{\text{term (A): Policy suboptimality}} + \underbrace{\mathbb{E}_{\theta \sim p(\theta)}[\sum_{k=1}^{K} \sum_{t=t_k}^{t_{k+1}-1} V^{\pi^t}_{\theta^k} (s_t) - V^{\pi^t}_\theta (s_t)]}_{\text{term(B): Model estimation gap}}
\end{align}
Term(A) in Eq. \ref{equ:regret_decomp_1} recalls the definition of $\epsilon$-optimality (eq. \ref{equ:eps_optim}), leading to:
\begin{equation}
    \text{term(A)} \le \epsilon T.
\end{equation}
Since LLM context is updated periodically, in the following we denote $\theta_k = \theta_t$ and $\pi^k = \pi^t$ for all $t \in \{t_k, t_k+1, ... t_{k+1}-1\}$.
For term(B) in Eq. \ref{equ:regret_decomp_1}, according to lemma C.1 in \cite{liu_reason_2023}, it can be decomposed into the information gain and value inconsistency, expressed as Eq. C.6 in \cite{liu_reason_2023}:
\begin{align}\label{equ:regret_decomp_2}
   &\frac{1-\gamma}{\gamma}\cdot\mathbb{E}_{\theta \sim p(\theta)}\Bigl[\sum_{k=0}^{K-1}\mathbb{E}_{\pi^k}\Bigl[\sum_{t=t_k}^{t_{k+1}-1} V_{\theta^k}^{\pi^k}(s_t)- V_{\theta}^{\pi^k}(s_t)\Bigr]\Bigr]\notag\\
   &\quad= \underbrace{\mathbb{E}_{\theta \sim p(\theta)}\Bigl[\sum_{k=0}^{K-1}\mathbb{E}_{\pi^k}\Bigl[\sum_{t=t_k}^{t_{k+1}-1} ({B}_{\theta^k}V^{\pi^k}_{\theta^k})(s_t,a_t) - ({B}_{\theta}V^{\pi^k}_{\theta^k})(s_t,a_t)\Bigr]\Bigr]}_{\text{term (C): information gain}}\notag\\
   &\quad\qquad +\underbrace{\mathbb{E}_{\theta \sim p(\theta)}\Bigl[\sum_{k=0}^{K-1}\mathbb{E}_{\pi^k}\Bigl[\bigl(V_{\theta^k}^{\pi^k}(s_{t_{k+1}}) - V^{\pi^k}_{\theta}(s_{t_{k+1}})\bigr)-\bigl(V_{\theta^k}^{\pi^k}(s_{t_k}) - V^{\pi^k}_{\theta}(s_{t_k}) \bigr) \Bigr]\Bigr]}_{\text{term (D): value inconsistency}},
\end{align}
where $B_\theta$ is the Bellman operator satisfying
\begin{equation}
    B_\theta V^\pi_\theta(s, a) = r_\theta(s, a) + \gamma P_\theta V^\pi_\theta(s, a).
\end{equation}
For term(C) in Eq. \ref{equ:regret_decomp_2}, recall Eq. \ref{equ:info_coeff} and Eq. C.10 in \cite{liu_reason_2023}, we have:
\begin{equation}
    \text{term(C)} \le \sup_{t^\dagger<T}\Gamma_{t^\dagger}(\delta)\cdot \mathbb{E}\bigl[\sqrt{ T (H_0 - H_{T}) }\bigr]+L\delta T
\end{equation}
For term(D) in Eq. \ref{equ:regret_decomp_2}, according to Eq. C.11 in \cite{liu_reason_2023}, we have
\begin{equation}
    \text{term (D)}\le {(4L/{\log2})\cdot\mathbb{E}[H_0 - H_{T}]}+4L\label{eq:b}.
\end{equation}
So Bayesian regret is bounded by (Theorem 4.4 in \cite{liu_reason_2023}):
\begin{equation}\label{equ:regret_order}
    \mathcal{R}(T) = O(\frac{\gamma \cdot (\sup_{t^\dagger<T}\Gamma_{t^\dagger}(\delta) \mathbb{E}\bigl[\sqrt{ (H_0 - H_{T}) }\bigr] \sqrt{T}  + L \delta T + L \mathbb{E}\bigl[\sqrt{ (H_0 - H_{T}) }\bigr])}{1-\gamma}  + \epsilon T)
\end{equation}
According to Eq. \ref{equ:regret_order}, if we have $\epsilon = O(\frac{1}{\sqrt{T}})$ and $\delta = O(\frac{1}{\sqrt{T}})$, then the whole term is essentially $O(\sqrt{T}).$

% \subsection{Proof of Lemma \ref{lem:offline_subo_bound}} \label{sec:proof_outer_loop}

% \subsection{Proof of Theorem \ref{thm:overall_result}} \label{sec:proof_overall}
